# Supplementary material for: Analysis of Contagion Dynamics with Active Cyber Defenders
Source: arXiv:2305.14694 source file (2023-05-24)
Supplement: Supplementary file 1 [file appendix.tex]

% !TEX root = main.tex
